# Supplementary material for: MotionScript: Natural Language Descriptions for Expressive 3D Human Motions
Source: arXiv:2312.12634 source file (2025-10-16)
Supplement: Supplementary file 1 [file appendix.tex]

\section*{Appendix}
\label{sec:appendix}

    \begin{table*}[]
        \footnotesize
        \begin{tabular}{@{}llll@{}}
        Posecode    & Axes and Ordinal Categories                                                             &  &  \\ \cmidrule(r){1-2}
        Orientation & x: lying flat forward,  leaning forward,  slightly leaning forward,  neutral ,  slightly leaning backward,  leaning backward,  lying flat backward                                                                                                                                        &  &  \\
                    & y: leaning left,  slightly leaning left,  slightly leaning right,  neutral,  slightly leaning right,  slightly leaning left,  leaning right                        &  &  \\
                    & z: about-face turned clockwise,  completely turned clockwise,  moderately turned clockwise,  slightly turned clockwise,  neutral,  &  &  \\
                    & slightly turned counter-clockwise, 
                     moderately turned counter-clockwise  completely turned counter-clockwise,  about-face turned counter-clockwise &  &  \\ \cmidrule(r){1-2}
        Translation & x: significant left,  left,  slightly left,   middle,  slightly right,  right,  significant right                                                                                                                                                                                        &  &  \\
                    & y: significant downward,  downward,  slightly downward,  middle, slightly upward,  upward,  significant upward                                                                                                                                                                          &  &  \\
                    & z: significant backward,  backward,  slightly backward,  middle,  slightly forward,  forward,  significant forward                                                                                                                                                                      &  & 
        \end{tabular}
        \caption{Introduced Posecodes. % for managing body rotations and translations Over Time. 
        % \textcolor{red}{This could be in Sup. materials...?}
        }
        
        \label{tab:posecode}
    \end{table*}
